# Supplementary material for: Variational quantum algorithms for local Hamiltonian problems
Source: arXiv:2208.11220 source file (2022-08-25)
Supplement: Supplementary file 1 [file appendix.tex]

\chapter{Примеры вставки листингов программного кода}\label{app:A}

Для крупных листингов есть два способа. Первый красивый, но в нём могут быть
проблемы с поддержкой кириллицы (у вас может встречаться в~комментариях
и~печатаемых сообщениях), он представлен на листинге~\cref{lst:hwbeauty}.
\begin{ListingEnv}[!h]% настройки floating аналогичны окружению figure
    \captiondelim{ } % разделитель идентификатора с номером от наименования
    \caption{Программа ,,Hello, world`` на \protect\cpp}\label{lst:hwbeauty}
    % окружение учитывает пробелы и табуляции и применяет их в сответсвии с настройками
    \begin{lstlisting}[language={[ISO]C++}]
	#include <iostream>
	using namespace std;

	int main() //кириллица в комментариях при xelatex и lualatex имеет проблемы с пробелами
	{
		cout << "Hello, world" << endl; //latin letters in commentaries
		system("pause");
		return 0;
	}
    \end{lstlisting}
\end{ListingEnv}%
Второй не~такой красивый, но без ограничений (см.~листинг~\cref{lst:hwplain}).
\begin{ListingEnv}[!h]
    \captiondelim{ } % разделитель идентификатора с номером от наименования
    \caption{Программа ,,Hello, world`` без подсветки}\label{lst:hwplain}
    \begin{Verb}

        #include <iostream>
        using namespace std;

        int main() //кириллица в комментариях
        {
            cout << "Привет, мир" << endl;
        }
    \end{Verb}
\end{ListingEnv}

Можно использовать первый для вставки небольших фрагментов
внутри текста, а второй для вставки полного
кода в приложении, если таковое имеется.

Если нужно вставить совсем короткий пример кода (одна или две строки),
то~выделение  линейками и нумерация может смотреться чересчур громоздко.
В таких случаях можно использовать окружения \texttt{lstlisting} или
\texttt{Verb} без \texttt{ListingEnv}. Приведём такой пример
с указанием языка программирования, отличного от~заданного по умолчанию:
\begin{lstlisting}[language=Haskell]
fibs = 0 : 1 : zipWith (+) fibs (tail fibs)
\end{lstlisting}
Такое решение "--- со вставкой нумерованных листингов покрупнее
и~вставок без выделения для маленьких фрагментов "--- выбрано,
например, в~книге Эндрю Таненбаума и Тодда Остина по архитектуре
компьютера.

Наконец, для оформления идентификаторов внутри строк
(функция \lstinline{main} и~тому подобное) используется
\texttt{lstinline} или, самое простое, моноширинный текст
(\texttt{\textbackslash texttt}).

Пример~\cref{lst:internal3}, иллюстрирующий подключение переопределённого
языка. Может быть полезным, если подсветка кода работает криво. Без
дополнительного окружения, с подписью и ссылкой, реализованной встроенным
средством.
\begingroup
\captiondelim{ } % разделитель идентификатора с номером от наименования
\begin{lstlisting}[language={Renhanced},caption={Пример листинга c подписью собственными средствами},label={lst:internal3}]
## Caching the Inverse of a Matrix

## Matrix inversion is usually a costly computation and there may be some
## benefit to caching the inverse of a matrix rather than compute it repeatedly
## This is a pair of functions that cache the inverse of a matrix.

## makeCacheMatrix creates a special "matrix" object that can cache its inverse

makeCacheMatrix <- function(x = matrix()) {#кириллица в комментариях при xelatex и lualatex имеет проблемы с пробелами
    i <- NULL
    set <- function(y) {
        x <<- y
        i <<- NULL
    }
    get <- function() x
    setSolved <- function(solve) i <<- solve
    getSolved <- function() i
    list(set = set, get = get,
    setSolved = setSolved,
    getSolved = getSolved)

}


## cacheSolve computes the inverse of the special "matrix" returned by
## makeCacheMatrix above. If the inverse has already been calculated (and the
## matrix has not changed), then the cachesolve should retrieve the inverse from
## the cache.

cacheSolve <- function(x, ...) {
    ## Return a matrix that is the inverse of 'x'
    i <- x$getSolved()
    if(!is.null(i)) {
        message("getting cached data")
        return(i)
    }
    data <- x$get()
    i <- solve(data, ...)
    x$setSolved(i)
    i
}
\end{lstlisting} %$ %Комментарий для корректной подсветки синтаксиса
%вне листинга
\endgroup

Листинг~\cref{lst:external1} подгружается из внешнего файла. Приходится
загружать без окружения дополнительного. Иначе по страницам не переносится.
\begingroup
\captiondelim{ } % разделитель идентификатора с номером от наименования
\lstinputlisting[lastline=78,language={R},caption={Листинг из внешнего файла},label={lst:external1}]{listings/run_analysis.R}
\endgroup

\chapter{Очень длинное название второго приложения, в~котором продемонстрирована работа с~длинными таблицами}\label{app:B}

\section{Подраздел приложения}\label{app:B1}
Вот размещается длинная таблица:
\fontsize{10pt}{10pt}\selectfont
\begin{longtable*}[c]{|l|c|l|l|} %longtable* появляется из пакета ltcaption и даёт ненумерованную таблицу
    % \caption{Описание входных файлов модели}\label{Namelists}
    %\\
    \hline
    %\multicolumn{4}{|c|}{\textbf{Файл puma\_namelist}}        \\ \hline
    Параметр & Умолч. & Тип & Описание               \\ \hline
    \endfirsthead   \hline
    \multicolumn{4}{|c|}{\small\slshape (продолжение)}        \\ \hline
    Параметр & Умолч. & Тип & Описание               \\ \hline
    \endhead        \hline
    % \multicolumn{4}{|c|}{\small\slshape (окончание)}        \\ \hline
    % Параметр & Умолч. & Тип & Описание               \\ \hline
    %                                             \endlasthead        \hline
    \multicolumn{4}{|r|}{\small\slshape продолжение следует}  \\ \hline
    \endfoot        \hline
    \endlastfoot
    \multicolumn{4}{|l|}{\&INP}        \\ \hline
    kick & 1 & int & 0: инициализация без шума (\(p_s = const\)) \\
    &   &     & 1: генерация белого шума                  \\
    &   &     & 2: генерация белого шума симметрично относительно \\
    & & & экватора    \\
    mars & 0 & int & 1: инициализация модели для планеты Марс     \\
    kick & 1 & int & 0: инициализация без шума (\(p_s = const\)) \\
    &   &     & 1: генерация белого шума                  \\
    &   &     & 2: генерация белого шума симметрично относительно \\
    & & & экватора    \\
    mars & 0 & int & 1: инициализация модели для планеты Марс     \\
    kick & 1 & int & 0: инициализация без шума (\(p_s = const\)) \\
    &   &     & 1: генерация белого шума                  \\
    &   &     & 2: генерация белого шума симметрично относительно \\
    & & & экватора    \\
    mars & 0 & int & 1: инициализация модели для планеты Марс     \\
    kick & 1 & int & 0: инициализация без шума (\(p_s = const\)) \\
    &   &     & 1: генерация белого шума                  \\
    &   &     & 2: генерация белого шума симметрично относительно \\
    & & & экватора    \\
    mars & 0 & int & 1: инициализация модели для планеты Марс     \\
    kick & 1 & int & 0: инициализация без шума (\(p_s = const\)) \\
    &   &     & 1: генерация белого шума                  \\
    &   &     & 2: генерация белого шума симметрично относительно \\
    & & & экватора    \\
    mars & 0 & int & 1: инициализация модели для планеты Марс     \\
    kick & 1 & int & 0: инициализация без шума (\(p_s = const\)) \\
    &   &     & 1: генерация белого шума                  \\
    &   &     & 2: генерация белого шума симметрично относительно \\
    & & & экватора    \\
    mars & 0 & int & 1: инициализация модели для планеты Марс     \\
    kick & 1 & int & 0: инициализация без шума (\(p_s = const\)) \\
    &   &     & 1: генерация белого шума                  \\
    &   &     & 2: генерация белого шума симметрично относительно \\
    & & & экватора    \\
    mars & 0 & int & 1: инициализация модели для планеты Марс     \\
    kick & 1 & int & 0: инициализация без шума (\(p_s = const\)) \\
    &   &     & 1: генерация белого шума                  \\
    &   &     & 2: генерация белого шума симметрично относительно \\
    & & & экватора    \\
    mars & 0 & int & 1: инициализация модели для планеты Марс     \\
    kick & 1 & int & 0: инициализация без шума (\(p_s = const\)) \\
    &   &     & 1: генерация белого шума                  \\
    &   &     & 2: генерация белого шума симметрично относительно \\
    & & & экватора    \\
    mars & 0 & int & 1: инициализация модели для планеты Марс     \\
    kick & 1 & int & 0: инициализация без шума (\(p_s = const\)) \\
    &   &     & 1: генерация белого шума                  \\
    &   &     & 2: генерация белого шума симметрично относительно \\
    & & & экватора    \\
    mars & 0 & int & 1: инициализация модели для планеты Марс     \\
    kick & 1 & int & 0: инициализация без шума (\(p_s = const\)) \\
    &   &     & 1: генерация белого шума                  \\
    &   &     & 2: генерация белого шума симметрично относительно \\
    & & & экватора    \\
    mars & 0 & int & 1: инициализация модели для планеты Марс     \\
    kick & 1 & int & 0: инициализация без шума (\(p_s = const\)) \\
    &   &     & 1: генерация белого шума                  \\
    &   &     & 2: генерация белого шума симметрично относительно \\
    & & & экватора    \\
    mars & 0 & int & 1: инициализация модели для планеты Марс     \\
    kick & 1 & int & 0: инициализация без шума (\(p_s = const\)) \\
    &   &     & 1: генерация белого шума                  \\
    &   &     & 2: генерация белого шума симметрично относительно \\
    & & & экватора    \\
    mars & 0 & int & 1: инициализация модели для планеты Марс     \\
    kick & 1 & int & 0: инициализация без шума (\(p_s = const\)) \\
    &   &     & 1: генерация белого шума                  \\
    &   &     & 2: генерация белого шума симметрично относительно \\
    & & & экватора    \\
    mars & 0 & int & 1: инициализация модели для планеты Марс     \\
    kick & 1 & int & 0: инициализация без шума (\(p_s = const\)) \\
    &   &     & 1: генерация белого шума                  \\
    &   &     & 2: генерация белого шума симметрично относительно \\
    & & & экватора    \\
    mars & 0 & int & 1: инициализация модели для планеты Марс     \\
    \hline
    %& & & \(\:\) \\
    \multicolumn{4}{|l|}{\&SURFPAR}        \\ \hline
    kick & 1 & int & 0: инициализация без шума (\(p_s = const\)) \\
    &   &     & 1: генерация белого шума                  \\
    &   &     & 2: генерация белого шума симметрично относительно \\
    & & & экватора    \\
    mars & 0 & int & 1: инициализация модели для планеты Марс     \\
    kick & 1 & int & 0: инициализация без шума (\(p_s = const\)) \\
    &   &     & 1: генерация белого шума                  \\
    &   &     & 2: генерация белого шума симметрично относительно \\
    & & & экватора    \\
    mars & 0 & int & 1: инициализация модели для планеты Марс     \\
    kick & 1 & int & 0: инициализация без шума (\(p_s = const\)) \\
    &   &     & 1: генерация белого шума                  \\
    &   &     & 2: генерация белого шума симметрично относительно \\
    & & & экватора    \\
    mars & 0 & int & 1: инициализация модели для планеты Марс     \\
    kick & 1 & int & 0: инициализация без шума (\(p_s = const\)) \\
    &   &     & 1: генерация белого шума                  \\
    &   &     & 2: генерация белого шума симметрично относительно \\
    & & & экватора    \\
    mars & 0 & int & 1: инициализация модели для планеты Марс     \\
    kick & 1 & int & 0: инициализация без шума (\(p_s = const\)) \\
    &   &     & 1: генерация белого шума                  \\
    &   &     & 2: генерация белого шума симметрично относительно \\
    & & & экватора    \\
    mars & 0 & int & 1: инициализация модели для планеты Марс     \\
    kick & 1 & int & 0: инициализация без шума (\(p_s = const\)) \\
    &   &     & 1: генерация белого шума                  \\
    &   &     & 2: генерация белого шума симметрично относительно \\
    & & & экватора    \\
    mars & 0 & int & 1: инициализация модели для планеты Марс     \\
    kick & 1 & int & 0: инициализация без шума (\(p_s = const\)) \\
    &   &     & 1: генерация белого шума                  \\
    &   &     & 2: генерация белого шума симметрично относительно \\
    & & & экватора    \\
    mars & 0 & int & 1: инициализация модели для планеты Марс     \\
    kick & 1 & int & 0: инициализация без шума (\(p_s = const\)) \\
    &   &     & 1: генерация белого шума                  \\
    &   &     & 2: генерация белого шума симметрично относительно \\
    & & & экватора    \\
    mars & 0 & int & 1: инициализация модели для планеты Марс     \\
    kick & 1 & int & 0: инициализация без шума (\(p_s = const\)) \\
    &   &     & 1: генерация белого шума                  \\
    &   &     & 2: генерация белого шума симметрично относительно \\
    & & & экватора    \\
    mars & 0 & int & 1: инициализация модели для планеты Марс     \\
    \hline
\end{longtable*}

\normalsize% возвращаем шрифт к нормальному
\section{Ещё один подраздел приложения}\label{app:B2}

Нужно больше подразделов приложения!
Конвынёры витюпырата но нам, тебиквюэ мэнтётюм позтюлант ед про. Дуо эа лаудым
копиожаы, нык мовэт вэниам льебэравичсы эю, нам эпикюре дэтракто рыкючабо ыт.

Пример длинной таблицы с записью продолжения по ГОСТ 2.105:

\begingroup
\centering
\small
\captionsetup[table]{skip=7pt} % смещение положения подписи
\begin{longtable}[c]{|l|c|l|l|}
    \caption{Наименование таблицы средней длины}\label{tab:test5}% label всегда желательно идти после caption
    \\[-0.45\onelineskip]
    \hline
    Параметр & Умолч. & Тип & Описание                                          \\ \hline
    \endfirsthead%
    \caption*{Продолжение таблицы~\thetable}                                    \\[-0.45\onelineskip]
    \hline
    Параметр & Умолч. & Тип & Описание                                          \\ \hline
    \endhead
    \hline
    \endfoot
    \hline
    \endlastfoot
    \multicolumn{4}{|l|}{\&INP}                                                 \\ \hline
    kick     & 1      & int & 0: инициализация без шума (\(p_s = const\))       \\
             &        &     & 1: генерация белого шума                          \\
             &        &     & 2: генерация белого шума симметрично относительно \\
             &        &     & экватора                                          \\
    mars     & 0      & int & 1: инициализация модели для планеты Марс          \\
    kick     & 1      & int & 0: инициализация без шума (\(p_s = const\))       \\
             &        &     & 1: генерация белого шума                          \\
             &        &     & 2: генерация белого шума симметрично относительно \\
             &        &     & экватора                                          \\
    mars     & 0      & int & 1: инициализация модели для планеты Марс          \\
    kick     & 1      & int & 0: инициализация без шума (\(p_s = const\))       \\
             &        &     & 1: генерация белого шума                          \\
             &        &     & 2: генерация белого шума симметрично относительно \\
             &        &     & экватора                                          \\
    mars     & 0      & int & 1: инициализация модели для планеты Марс          \\
    kick     & 1      & int & 0: инициализация без шума (\(p_s = const\))       \\
             &        &     & 1: генерация белого шума                          \\
             &        &     & 2: генерация белого шума симметрично относительно \\
             &        &     & экватора                                          \\
    mars     & 0      & int & 1: инициализация модели для планеты Марс          \\
    kick     & 1      & int & 0: инициализация без шума (\(p_s = const\))       \\
             &        &     & 1: генерация белого шума                          \\
             &        &     & 2: генерация белого шума симметрично относительно \\
             &        &     & экватора                                          \\
    mars     & 0      & int & 1: инициализация модели для планеты Марс          \\
    kick     & 1      & int & 0: инициализация без шума (\(p_s = const\))       \\
             &        &     & 1: генерация белого шума                          \\
             &        &     & 2: генерация белого шума симметрично относительно \\
             &        &     & экватора                                          \\
    mars     & 0      & int & 1: инициализация модели для планеты Марс          \\
    kick     & 1      & int & 0: инициализация без шума (\(p_s = const\))       \\
             &        &     & 1: генерация белого шума                          \\
             &        &     & 2: генерация белого шума симметрично относительно \\
             &        &     & экватора                                          \\
    mars     & 0      & int & 1: инициализация модели для планеты Марс          \\
    kick     & 1      & int & 0: инициализация без шума (\(p_s = const\))       \\
             &        &     & 1: генерация белого шума                          \\
             &        &     & 2: генерация белого шума симметрично относительно \\
             &        &     & экватора                                          \\
    mars     & 0      & int & 1: инициализация модели для планеты Марс          \\
    kick     & 1      & int & 0: инициализация без шума (\(p_s = const\))       \\
             &        &     & 1: генерация белого шума                          \\
             &        &     & 2: генерация белого шума симметрично относительно \\
             &        &     & экватора                                          \\
    mars     & 0      & int & 1: инициализация модели для планеты Марс          \\
    kick     & 1      & int & 0: инициализация без шума (\(p_s = const\))       \\
             &        &     & 1: генерация белого шума                          \\
             &        &     & 2: генерация белого шума симметрично относительно \\
             &        &     & экватора                                          \\
    mars     & 0      & int & 1: инициализация модели для планеты Марс          \\
    kick     & 1      & int & 0: инициализация без шума (\(p_s = const\))       \\
             &        &     & 1: генерация белого шума                          \\
             &        &     & 2: генерация белого шума симметрично относительно \\
             &        &     & экватора                                          \\
    mars     & 0      & int & 1: инициализация модели для планеты Марс          \\
    kick     & 1      & int & 0: инициализация без шума (\(p_s = const\))       \\
             &        &     & 1: генерация белого шума                          \\
             &        &     & 2: генерация белого шума симметрично относительно \\
             &        &     & экватора                                          \\
    mars     & 0      & int & 1: инициализация модели для планеты Марс          \\
    kick     & 1      & int & 0: инициализация без шума (\(p_s = const\))       \\
             &        &     & 1: генерация белого шума                          \\
             &        &     & 2: генерация белого шума симметрично относительно \\
             &        &     & экватора                                          \\
    mars     & 0      & int & 1: инициализация модели для планеты Марс          \\
    kick     & 1      & int & 0: инициализация без шума (\(p_s = const\))       \\
             &        &     & 1: генерация белого шума                          \\
             &        &     & 2: генерация белого шума симметрично относительно \\
             &        &     & экватора                                          \\
    mars     & 0      & int & 1: инициализация модели для планеты Марс          \\
    kick     & 1      & int & 0: инициализация без шума (\(p_s = const\))       \\
             &        &     & 1: генерация белого шума                          \\
             &        &     & 2: генерация белого шума симметрично относительно \\
             &        &     & экватора                                          \\
    mars     & 0      & int & 1: инициализация модели для планеты Марс          \\
    \hline
    %& & & $\:$ \\
    \multicolumn{4}{|l|}{\&SURFPAR}                                             \\ \hline
    kick     & 1      & int & 0: инициализация без шума (\(p_s = const\))       \\
             &        &     & 1: генерация белого шума                          \\
             &        &     & 2: генерация белого шума симметрично относительно \\
             &        &     & экватора                                          \\
    mars     & 0      & int & 1: инициализация модели для планеты Марс          \\
    kick     & 1      & int & 0: инициализация без шума (\(p_s = const\))       \\
             &        &     & 1: генерация белого шума                          \\
             &        &     & 2: генерация белого шума симметрично относительно \\
             &        &     & экватора                                          \\
    mars     & 0      & int & 1: инициализация модели для планеты Марс          \\
    kick     & 1      & int & 0: инициализация без шума (\(p_s = const\))       \\
             &        &     & 1: генерация белого шума                          \\
             &        &     & 2: генерация белого шума симметрично относительно \\
             &        &     & экватора                                          \\
    mars     & 0      & int & 1: инициализация модели для планеты Марс          \\
    kick     & 1      & int & 0: инициализация без шума (\(p_s = const\))       \\
             &        &     & 1: генерация белого шума                          \\
             &        &     & 2: генерация белого шума симметрично относительно \\
             &        &     & экватора                                          \\
    mars     & 0      & int & 1: инициализация модели для планеты Марс          \\
    kick     & 1      & int & 0: инициализация без шума (\(p_s = const\))       \\
             &        &     & 1: генерация белого шума                          \\
             &        &     & 2: генерация белого шума симметрично относительно \\
             &        &     & экватора                                          \\
    mars     & 0      & int & 1: инициализация модели для планеты Марс          \\
    kick     & 1      & int & 0: инициализация без шума (\(p_s = const\))       \\
             &        &     & 1: генерация белого шума                          \\
             &        &     & 2: генерация белого шума симметрично относительно \\
             &        &     & экватора                                          \\
    mars     & 0      & int & 1: инициализация модели для планеты Марс          \\
    kick     & 1      & int & 0: инициализация без шума (\(p_s = const\))       \\
             &        &     & 1: генерация белого шума                          \\
             &        &     & 2: генерация белого шума симметрично относительно \\
             &        &     & экватора                                          \\
    mars     & 0      & int & 1: инициализация модели для планеты Марс          \\
    kick     & 1      & int & 0: инициализация без шума (\(p_s = const\))       \\
             &        &     & 1: генерация белого шума                          \\
             &        &     & 2: генерация белого шума симметрично относительно \\
             &        &     & экватора                                          \\
    mars     & 0      & int & 1: инициализация модели для планеты Марс          \\
    kick     & 1      & int & 0: инициализация без шума (\(p_s = const\))       \\
             &        &     & 1: генерация белого шума                          \\
             &        &     & 2: генерация белого шума симметрично относительно \\
             &        &     & экватора                                          \\
    mars     & 0      & int & 1: инициализация модели для планеты Марс          \\
\end{longtable}
\normalsize% возвращаем шрифт к нормальному
\endgroup
\section{Использование длинных таблиц с окружением \textit{longtabu}}\label{app:B2a}

В таблице \cref{tab:test-functions} более книжный вариант
длинной таблицы, используя окружение \verb!longtabu! и разнообразные
\verb!toprule! \verb!midrule! \verb!bottomrule! из~пакета
\verb!booktabs!. Чтобы визуально таблица смотрелась лучше, можно
использовать следующие параметры: в самом начале задаётся расстояние
между строчками с~помощью \verb!arraystretch!. Таблица задаётся на
всю ширину, \verb!longtabu! позволяет делить ширину колонок
пропорционально "--- тут три колонки в~пропорции 1.1:1:4 "--- для каждой
колонки первый параметр в~описании \verb!X[]!. Кроме того, в~таблице
убраны отступы слева и справа с~помощью \verb!@{}!
в~преамбуле таблицы. К~первому и~второму столбцу применяется
модификатор

\verb!>{\setlength{\baselineskip}{0.7\baselineskip}}!,

\noindent который уменьшает межстрочный интервал в для текста таблиц (иначе
заголовок второго столбца значительно шире, а двухстрочное имя
сливается с~окружающими). Для первой и второй колонки текст в ячейках
выравниваются по~центру как по~вертикали, так и по горизонтали "---
задаётся буквами \verb!m!~и~\verb!c!~в~описании столбца \verb!X[]!.

Так как формулы большие "--- используется окружение \verb!alignedat!,
чтобы отступ был одинаковый у всех формул "--- он сделан для всех, хотя
для большей части можно было и не использовать.  Чтобы формулы
занимали поменьше места в~каждом столбце формулы (где надо)
используется \verb!\textstyle! "--- он~делает дроби меньше, у~знаков
суммы и произведения "--- индексы сбоку. Иногда формула слишком большая,
сливается со следующей, поэтому после неё ставится небольшой
дополнительный отступ \verb!\vspace*{2ex}!. Для штрафных функций "---
размер фигурных скобок задан вручную \verb!\Big\{!, т.\:к. не~умеет
\verb!alignedat! работать с~\verb!\left! и~\verb!\right! через
несколько строк/колонок.

В примечании к таблице наоборот, окружение \verb!cases! даёт слишком
большие промежутки между вариантами, чтобы их уменьшить, в конце
каждой строчки окружения использовался отрицательный дополнительный
отступ \verb!\\[-0.5em]!.

\begingroup % Ограничиваем область видимости arraystretch
%% Увеличение расстояния между рядами, для улучшения восприятия.
\begin{longtabu} to \textwidth
    {%
    @{}>{\setlength{\baselineskip}{0.7\baselineskip}}X[1.1mc]%
    >{\setlength{\baselineskip}{0.7\baselineskip}}X[1.1mc]%
    X[4]@{}%
    }
    \caption{Тестовые функции для оптимизации, \(D\) "---
        размерность. Для всех функций значение в точке глобального
        минимума равно нулю.\label{tab:test-functions}}\\% label всегда желательно идти после caption

    \toprule     %%% верхняя линейка
    Имя           &Стартовый диапазон параметров &Функция  \\
    \midrule %%% тонкий разделитель. Отделяет названия столбцов. Обязателен по ГОСТ 2.105 пункт 4.4.5
    \endfirsthead

    \multicolumn{3}{c}{\small\slshape (продолжение)}        \\
    \toprule     %%% верхняя линейка
    Имя           &Стартовый диапазон параметров &Функция  \\
    \midrule %%% тонкий разделитель. Отделяет названия столбцов. Обязателен по ГОСТ 2.105 пункт 4.4.5
    \endhead

    \multicolumn{3}{c}{\small\slshape (окончание)}        \\
    \toprule     %%% верхняя линейка
    Имя           &Стартовый диапазон параметров &Функция  \\
    \midrule %%% тонкий разделитель. Отделяет названия столбцов. Обязателен по ГОСТ 2.105 пункт 4.4.5
    \endlasthead

    \bottomrule %%% нижняя линейка
    \multicolumn{3}{r}{\small\slshape продолжение следует}  \\
    \endfoot
    \endlastfoot

    сфера         &\(\left[-100,\,100\right]^D\)   &
    \(\begin{aligned}
        \textstyle f_1(x)=\sum_{i=1}^Dx_i^2
    \end{aligned}\) \\
    Schwefel 2.22 &\(\left[-10,\,10\right]^D\)     &
    \(\begin{aligned}
        \textstyle f_2(x)=\sum_{i=1}^D|x_i|+\prod_{i=1}^D|x_i|
    \end{aligned}\) \\
    Schwefel 1.2  &\(\left[-100,\,100\right]^D\)   &
    \(\begin{aligned}
        \textstyle f_3(x)=\sum_{i=1}^D\left(\sum_{j=1}^ix_j\right)^2
    \end{aligned}\) \\
    Schwefel 2.21 &\(\left[-100,\,100\right]^D\)   &
    \(\begin{aligned}
        \textstyle f_4(x)=\max_i\!\left\{\left|x_i\right|\right\}
    \end{aligned}\) \\
    Rosenbrock    &\(\left[-30,\,30\right]^D\)     &
    \(\begin{aligned}
        \textstyle f_5(x)=
        \sum_{i=1}^{D-1}
        \left[100\!\left(x_{i+1}-x_i^2\right)^2+(x_i-1)^2\right]
    \end{aligned}\) \\
    ступенчатая   &\(\left[-100,\,100\right]^D\)   &
    \(\begin{aligned}
        \textstyle f_6(x)=\sum_{i=1}^D\big\lfloor x_i+0.5\big\rfloor^2
    \end{aligned}\) \\
    зашумлённая квартическая &\(\left[-1.28,\,1.28\right]^D\) &
    \(\begin{aligned}
        \textstyle f_7(x)=\sum_{i=1}^Dix_i^4+rand[0,1)
    \end{aligned}\)\vspace*{2ex}\\
    Schwefel 2.26 &\(\left[-500,\,500\right]^D\)   &
    \(\begin{aligned}
        f_8(x)= & \textstyle\sum_{i=1}^D-x_i\,\sin\sqrt{|x_i|}\,+ \\
                & \vphantom{\sum}+ D\cdot
        418.98288727243369
    \end{aligned}\)\\
    Rastrigin     &\(\left[-5.12,\,5.12\right]^D\) &
    \(\begin{aligned}
        \textstyle f_9(x)=\sum_{i=1}^D\left[x_i^2-10\,\cos(2\pi x_i)+10\right]
    \end{aligned}\)\vspace*{2ex}\\
    Ackley        &\(\left[-32,\,32\right]^D\)     &
    \(\begin{aligned}
        f_{10}(x)= & \textstyle -20\, \exp\!\left(
        -0.2\sqrt{\frac{1}{D}\sum_{i=1}^Dx_i^2} \right)- \\
                   & \textstyle - \exp\left(
            \frac{1}{D}\sum_{i=1}^D\cos(2\pi x_i)  \right)
        + 20 + e
    \end{aligned}\) \\
    Griewank      &\(\left[-600,\,600\right]^D\) &
    \(\begin{aligned}
        f_{11}(x)= & \textstyle \frac{1}{4000}\sum_{i=1}^{D}x_i^2 -
        \prod_{i=1}^D\cos\left(x_i/\sqrt{i}\right) +1
    \end{aligned}\) \vspace*{3ex} \\
    штрафная 1    &\(\left[-50,\,50\right]^D\)     &
    \(\begin{aligned}
        f_{12}(x)= & \textstyle \frac{\pi}{D}\Big\{ 10\,\sin^2(\pi y_1) +            \\
                   & +\textstyle \sum_{i=1}^{D-1}(y_i-1)^2
        \left[1+10\,\sin^2(\pi y_{i+1})\right] +                                     \\
                   & +(y_D-1)^2 \Big\} +\textstyle\sum_{i=1}^D u(x_i,\,10,\,100,\,4)
    \end{aligned}\) \vspace*{2ex} \\
    штрафная 2    &\(\left[-50,\,50\right]^D\)     &
    \(\begin{aligned}
        f_{13}(x)= & \textstyle 0.1 \Big\{\sin^2(3\pi x_1) +            \\
                   & +\textstyle \sum_{i=1}^{D-1}(x_i-1)^2
        \left[1+\sin^2(3 \pi x_{i+1})\right] +                          \\
                   & +(x_D-1)^2\left[1+\sin^2(2\pi x_D)\right] \Big\} + \\
                   & +\textstyle\sum_{i=1}^D u(x_i,\,5,\,100,\,4)
    \end{aligned}\)\\
    сфера         &\(\left[-100,\,100\right]^D\)   &
    \(\begin{aligned}
        \textstyle f_1(x)=\sum_{i=1}^Dx_i^2
    \end{aligned}\) \\
    Schwefel 2.22 &\(\left[-10,\,10\right]^D\)     &
    \(\begin{aligned}
        \textstyle f_2(x)=\sum_{i=1}^D|x_i|+\prod_{i=1}^D|x_i|
    \end{aligned}\) \\
    Schwefel 1.2  &\(\left[-100,\,100\right]^D\)   &
    \(\begin{aligned}
        \textstyle f_3(x)=\sum_{i=1}^D\left(\sum_{j=1}^ix_j\right)^2
    \end{aligned}\) \\
    Schwefel 2.21 &\(\left[-100,\,100\right]^D\)   &
    \(\begin{aligned}
        \textstyle f_4(x)=\max_i\!\left\{\left|x_i\right|\right\}
    \end{aligned}\) \\
    Rosenbrock    &\(\left[-30,\,30\right]^D\)     &
    \(\begin{aligned}
        \textstyle f_5(x)=
        \sum_{i=1}^{D-1}
        \left[100\!\left(x_{i+1}-x_i^2\right)^2+(x_i-1)^2\right]
    \end{aligned}\) \\
    ступенчатая   &\(\left[-100,\,100\right]^D\)   &
    \(\begin{aligned}
        \textstyle f_6(x)=\sum_{i=1}^D\big\lfloor x_i+0.5\big\rfloor^2
    \end{aligned}\) \\
    зашумлённая квартическая &\(\left[-1.28,\,1.28\right]^D\) &
    \(\begin{aligned}
        \textstyle f_7(x)=\sum_{i=1}^Dix_i^4+rand[0,1)
    \end{aligned}\)\vspace*{2ex}\\
    Schwefel 2.26 &\(\left[-500,\,500\right]^D\)   &
    \(\begin{aligned}
        f_8(x)= & \textstyle\sum_{i=1}^D-x_i\,\sin\sqrt{|x_i|}\,+ \\
                & \vphantom{\sum}+ D\cdot
        418.98288727243369
    \end{aligned}\)\\
    Rastrigin     &\(\left[-5.12,\,5.12\right]^D\) &
    \(\begin{aligned}
        \textstyle f_9(x)=\sum_{i=1}^D\left[x_i^2-10\,\cos(2\pi x_i)+10\right]
    \end{aligned}\)\vspace*{2ex}\\
    Ackley        &\(\left[-32,\,32\right]^D\)     &
    \(\begin{aligned}
        f_{10}(x)= & \textstyle -20\, \exp\!\left(
        -0.2\sqrt{\frac{1}{D}\sum_{i=1}^Dx_i^2} \right)- \\
                   & \textstyle - \exp\left(
            \frac{1}{D}\sum_{i=1}^D\cos(2\pi x_i)  \right)
        + 20 + e
    \end{aligned}\) \\
    Griewank      &\(\left[-600,\,600\right]^D\) &
    \(\begin{aligned}
        f_{11}(x)= & \textstyle \frac{1}{4000}\sum_{i=1}^{D}x_i^2 -
        \prod_{i=1}^D\cos\left(x_i/\sqrt{i}\right) +1
    \end{aligned}\) \vspace*{3ex} \\
    штрафная 1    &\(\left[-50,\,50\right]^D\)     &
    \(\begin{aligned}
        f_{12}(x)= & \textstyle \frac{\pi}{D}\Big\{ 10\,\sin^2(\pi y_1) +            \\
                   & +\textstyle \sum_{i=1}^{D-1}(y_i-1)^2
        \left[1+10\,\sin^2(\pi y_{i+1})\right] +                                     \\
                   & +(y_D-1)^2 \Big\} +\textstyle\sum_{i=1}^D u(x_i,\,10,\,100,\,4)
    \end{aligned}\) \vspace*{2ex} \\
    штрафная 2    &\(\left[-50,\,50\right]^D\)     &
    \(\begin{aligned}
        f_{13}(x)= & \textstyle 0.1 \Big\{\sin^2(3\pi x_1) +            \\
                   & +\textstyle \sum_{i=1}^{D-1}(x_i-1)^2
        \left[1+\sin^2(3 \pi x_{i+1})\right] +                          \\
                   & +(x_D-1)^2\left[1+\sin^2(2\pi x_D)\right] \Big\} + \\
                   & +\textstyle\sum_{i=1}^D u(x_i,\,5,\,100,\,4)
    \end{aligned}\)\\
    \midrule%%% тонкий разделитель
    \multicolumn{3}{@{}p{\textwidth}}{%
    \vspace*{-3.5ex}% этим подтягиваем повыше
    \hspace*{2.5em}% абзацный отступ - требование ГОСТ 2.105
    Примечание "---  Для функций \(f_{12}\) и \(f_{13}\)
    используется \(y_i = 1 + \frac{1}{4}(x_i+1)\)
    и~$u(x_i,\,a,\,k,\,m)=
        \begin{cases*}
            k(x_i-a)^m,  & \( x_i >a \)            \\[-0.5em]
            0,           & \( -a\leq x_i \leq a \) \\[-0.5em]
            k(-x_i-a)^m, & \( x_i <-a \)
        \end{cases*}
    $
    }\\
    \bottomrule %%% нижняя линейка
\end{longtabu}
\endgroup

\section{Форматирование внутри таблиц}\label{app:B3}

В таблице \cref{tab:other-row} пример с чересстрочным
форматированием. В~файле \verb+userstyles.tex+  задаётся счётчик
\verb+\newcounter{rowcnt}+ который увеличивается на~1 после каждой
строчки (как указано в преамбуле таблицы). Кроме того, задаётся
условный макрос \verb+\altshape+ который выдаёт одно
из~двух типов форматирования в~зависимости от чётности счётчика.

В таблице \cref{tab:other-row} каждая чётная строчка "--- синяя,
нечётная "--- с наклоном и~слегка поднята вверх. Визуально это приводит
к тому, что среднее значение и~среднеквадратичное изменение
группируются и хорошо выделяются взглядом в~таблице. Сохраняется
возможность отдельные значения в таблице выделить цветом или
шрифтом. К первому и второму столбцу форматирование не применяется
по~сути таблицы, к шестому общее форматирование не~применяется для
наглядности.

Так как заголовок таблицы тоже считается за строчку, то перед ним (для
первого, промежуточного и финального варианта) счётчик обнуляется,
а~в~\verb+\altshape+ для нулевого значения счётчика форматирования
не~применяется.

\begingroup % Ограничиваем область видимости arraystretch
\renewcommand\altshape{
    \ifnumequal{\value{rowcnt}}{0}{
        % Стиль для заголовка таблицы
    }{
        \ifnumodd{\value{rowcnt}}
        {
            \color{blue} % Cтиль для нечётных строк
        }{
            \vspace*{-0.7ex}\itshape} % Стиль для чётных строк
    }
}
\newcolumntype{A}{>{\centering\begingroup\altshape}X[1mc]<{\endgroup}}
\needspace{2\baselineskip}
%% Уменьшаем  расстояние между
%% рядами, чтобы таблица не так много
%% места занимала в дисере.
\begin{longtabu} to \textwidth {@{}X[0.27ml]@{}X[0.7mc]@{}A@{}A@{}A@{}X[0.98mc]@{}>{\setlength{\baselineskip}{0.7\baselineskip}}A@{}A<{\stepcounter{rowcnt}}@{}}
    % \begin{longtabu} to \textwidth {@{}X[0.2ml]X[1mc]X[1mc]X[1mc]X[1mc]X[1mc]>{\setlength{\baselineskip}{0.7\baselineskip}}X[1mc]X[1mc]@{}}
    \caption{Длинная таблица с примером чересстрочного форматирования\label{tab:other-row}}\vspace*{1ex}\\% label всегда желательно идти после caption
    % \vspace*{1ex}     \\

    \toprule %%% верхняя линейка
    \setcounter{rowcnt}{0} &Итера\-ции & JADE\texttt{++} & JADE & jDE & SaDE
    & DE/rand /1/bin & PSO \\
    \midrule %%% тонкий разделитель. Отделяет названия столбцов. Обязателен по ГОСТ 2.105 пункт 4.4.5
    \endfirsthead

    \multicolumn{8}{c}{\small\slshape (продолжение)} \\
    \toprule %%% верхняя линейка
    \setcounter{rowcnt}{0} &Итера\-ции & JADE\texttt{++} & JADE & jDE & SaDE
    & DE/rand /1/bin & PSO \\
    \midrule %%% тонкий разделитель. Отделяет названия столбцов. Обязателен по ГОСТ 2.105 пункт 4.4.5
    \endhead

    \multicolumn{8}{c}{\small\slshape (окончание)} \\
    \toprule %%% верхняя линейка
    \setcounter{rowcnt}{0} &Итера\-ции & JADE\texttt{++} & JADE & jDE & SaDE
    & DE/rand /1/bin & PSO \\
    \midrule %%% тонкий разделитель. Отделяет названия столбцов. Обязателен по ГОСТ 2.105 пункт 4.4.5
    \endlasthead

    \bottomrule %%% нижняя линейка
    \multicolumn{8}{r}{\small\slshape продолжение следует}     \\
    \endfoot
    \endlastfoot

    f1  & 1500 & \textbf{1.8E-60}   & 1.3E-54   & 2.5E-28   & 4.5E-20   & 9.8E-14   & 9.6E-42   \\\nopagebreak
    &      & (8.4E-60) & (9.2E-54) & {\color{red}(3.5E-28)} & (6.9E-20) & (8.4E-14) & (2.7E-41) \\
    f2  & 2000 & 1.8E-25   & 3.9E-22   & 1.5E-23   & 1.9E-14   & 1.6E-09   & 9.3E-21   \\\nopagebreak
    &      & (8.8E-25) & (2.7E-21) & (1.0E-23) & (1.1E-14) & (1.1E-09) & (6.3E-20) \\
    f3  & 5000 & 5.7E-61   & 6.0E-87   & 5.2E-14   & {\color{green}9.0E-37}   & 6.6E-11   & 2.5E-19   \\\nopagebreak
    &      & (2.7E-60) & (1.9E-86) & (1.1E-13) & (5.4E-36) & (8.8E-11) & (3.9E-19) \\
    f4  & 5000 & 8.2E-24   & 4.3E-66   & 1.4E-15   & 7.4E-11   & 4.2E-01   & 4.4E-14   \\\nopagebreak
    &      & (4.0E-23) & (1.2E-65) & (1.0E-15) & (1.8E-10) & (1.1E+00) & (9.3E-14) \\
    f5  & 3000 & 8.0E-02   & 3.2E-01   & 1.3E+01   & 2.1E+01   & 2.1E+00   & 2.5E+01   \\\nopagebreak
    &      & (5.6E-01) & (1.1E+00) & (1.4E+01) & (7.8E+00) & (1.5E+00) & (3.2E+01) \\
    f6  & 100  & 2.9E+00   & 5.6E+00   & 1.0E+03   & 9.3E+02   & 4.7E+03   & 4.5E+01   \\\nopagebreak
    &      & (1.2E+00) & (1.6E+00) & (2.2E+02) & (1.8E+02) & (1.1E+03) & (2.4E+01) \\
    f7  & 3000 & 6.4E-04   & 6.8E-04   & 3.3E-03   & 4.8E-03   & 4.7E-03   & 2.5E-03   \\\nopagebreak
    &      & (2.5E-04) & (2.5E-04) & (8.5E-04) & (1.2E-03) & (1.2E-03) & (1.4E-03) \\
    f8  & 1000 & 3.3E-05   & 7.1E+00   & 7.9E-11   & 4.7E+00   & 5.9E+03   & 2.4E+03   \\\nopagebreak
    &      & (2.3E-05) & (2.8E+01) & (1.3E-10) & (3.3E+01) & (1.1E+03) & (6.7E+02) \\
    f9  & 1000 & 1.0E-04   & 1.4E-04   & 1.5E-04   & 1.2E-03   & 1.8E+02   & 5.2E+01   \\\nopagebreak
    &      & (6.0E-05) & (6.5E-05) & (2.0E-04) & (6.5E-04) & (1.3E+01) & (1.6E+01) \\
    f10 & 500  & 8.2E-10   & 3.0E-09   & 3.5E-04   & 2.7E-03   & 1.1E-01   & 4.6E-01   \\\nopagebreak
    &      & (6.9E-10) & (2.2E-09) & (1.0E-04) & (5.1E-04) & (3.9E-02) & (6.6E-01) \\
    f11 & 500  & 9.9E-08   & 2.0E-04   & 1.9E-05   & 7.8E-04  & 2.0E-01   & 1.3E-02   \\\nopagebreak
    &      & (6.0E-07) & (1.4E-03) & (5.8E-05) & (1.2E-03)  & (1.1E-01) & (1.7E-02) \\
    f12 & 500  & 4.6E-17   & 3.8E-16   & 1.6E-07   & 1.9E-05   & 1.2E-02   & 1.9E-01   \\\nopagebreak
    &      & (1.9E-16) & (8.3E-16) & (1.5E-07) & (9.2E-06) & (1.0E-02) & (3.9E-01) \\
    f13 & 500  & 2.0E-16   & 1.2E-15   & 1.5E-06   & 6.1E-05   & 7.5E-02   & 2.9E-03   \\\nopagebreak
    &      & (6.5E-16) & (2.8E-15) & (9.8E-07) & (2.0E-05) & (3.8E-02) & (4.8E-03) \\
    f1  & 1500 & \textbf{1.8E-60}   & 1.3E-54   & 2.5E-28   & 4.5E-20   & 9.8E-14   & 9.6E-42   \\\nopagebreak
    &      & (8.4E-60) & (9.2E-54) & {\color{red}(3.5E-28)} & (6.9E-20) & (8.4E-14) & (2.7E-41) \\
    f2  & 2000 & 1.8E-25   & 3.9E-22   & 1.5E-23   & 1.9E-14   & 1.6E-09   & 9.3E-21   \\\nopagebreak
    &      & (8.8E-25) & (2.7E-21) & (1.0E-23) & (1.1E-14) & (1.1E-09) & (6.3E-20) \\
    f3  & 5000 & 5.7E-61   & 6.0E-87   & 5.2E-14   & 9.0E-37   & 6.6E-11   & 2.5E-19   \\\nopagebreak
    &      & (2.7E-60) & (1.9E-86) & (1.1E-13) & (5.4E-36) & (8.8E-11) & (3.9E-19) \\
    f4  & 5000 & 8.2E-24   & 4.3E-66   & 1.4E-15   & 7.4E-11   & 4.2E-01   & 4.4E-14   \\\nopagebreak
    &      & (4.0E-23) & (1.2E-65) & (1.0E-15) & (1.8E-10) & (1.1E+00) & (9.3E-14) \\
    f5  & 3000 & 8.0E-02   & 3.2E-01   & 1.3E+01   & 2.1E+01   & 2.1E+00   & 2.5E+01   \\\nopagebreak
    &      & (5.6E-01) & (1.1E+00) & (1.4E+01) & (7.8E+00) & (1.5E+00) & (3.2E+01) \\
    f6  & 100  & 2.9E+00   & 5.6E+00   & 1.0E+03   & 9.3E+02   & 4.7E+03   & 4.5E+01   \\\nopagebreak
    &      & (1.2E+00) & (1.6E+00) & (2.2E+02) & (1.8E+02) & (1.1E+03) & (2.4E+01) \\
    f7  & 3000 & 6.4E-04   & 6.8E-04   & 3.3E-03   & 4.8E-03   & 4.7E-03   & 2.5E-03   \\\nopagebreak
    &      & (2.5E-04) & (2.5E-04) & (8.5E-04) & (1.2E-03) & (1.2E-03) & (1.4E-03) \\
    f8  & 1000 & 3.3E-05   & 7.1E+00   & 7.9E-11   & 4.7E+00   & 5.9E+03   & 2.4E+03   \\\nopagebreak
    &      & (2.3E-05) & (2.8E+01) & (1.3E-10) & (3.3E+01) & (1.1E+03) & (6.7E+02) \\
    f9  & 1000 & 1.0E-04   & 1.4E-04   & 1.5E-04   & 1.2E-03   & 1.8E+02   & 5.2E+01   \\\nopagebreak
    &      & (6.0E-05) & (6.5E-05) & (2.0E-04) & (6.5E-04) & (1.3E+01) & (1.6E+01) \\
    f10 & 500  & 8.2E-10   & 3.0E-09   & 3.5E-04   & 2.7E-03   & 1.1E-01   & 4.6E-01   \\\nopagebreak
    &      & (6.9E-10) & (2.2E-09) & (1.0E-04) & (5.1E-04) & (3.9E-02) & (6.6E-01) \\
    f11 & 500  & 9.9E-08   & 2.0E-04   & 1.9E-05   & 7.8E-04  & 2.0E-01   & 1.3E-02   \\\nopagebreak
    &      & (6.0E-07) & (1.4E-03) & (5.8E-05) & (1.2E-03)  & (1.1E-01) & (1.7E-02) \\
    f12 & 500  & 4.6E-17   & 3.8E-16   & 1.6E-07   & 1.9E-05   & 1.2E-02   & 1.9E-01   \\\nopagebreak
    &      & (1.9E-16) & (8.3E-16) & (1.5E-07) & (9.2E-06) & (1.0E-02) & (3.9E-01) \\
    f13 & 500  & 2.0E-16   & 1.2E-15   & 1.5E-06   & 6.1E-05   & 7.5E-02   & 2.9E-03   \\\nopagebreak
    &      & (6.5E-16) & (2.8E-15) & (9.8E-07) & (2.0E-05) & (3.8E-02) & (4.8E-03) \\
    \bottomrule %%% нижняя линейка
\end{longtabu} \endgroup

\section{Стандартные префиксы ссылок}\label{app:B4}

Общепринятым является следующий формат ссылок: \texttt{<prefix>:<label>}.
Например, \verb+\label{fig:knuth}+; \verb+\ref{tab:test1}+; \verb+label={lst:external1}+.
В~таблице \cref{tab:tab_pref} приведены стандартные префиксы для различных
типов ссылок.

\begin{table}[htbp]
    \captionsetup{justification=centering}
    \centering{
        \caption{\label{tab:tab_pref}Стандартные префиксы ссылок}
        \begin{tabular}{ll}
            \toprule
            \textbf{Префикс} & \textbf{Описание} \\
            \midrule
            ch:              & Глава             \\
            sec:             & Секция            \\
            subsec:          & Подсекция         \\
            fig:             & Рисунок           \\
            tab:             & Таблица           \\
            eq:              & Уравнение         \\
            lst:             & Листинг программы \\
            itm:             & Элемент списка    \\
            alg:             & Алгоритм          \\
            app:             & Секция приложения \\
            \bottomrule
        \end{tabular}
    }
\end{table}

Для упорядочивания ссылок можно использовать разделительные символы.
Например, \verb+\label{fig:scheemes/my_scheeme}+ или \\ \verb+\label{lst:dts/linked_list}+.

\section{Очередной подраздел приложения}\label{app:B5}

Нужно больше подразделов приложения!

\section{И ещё один подраздел приложения}\label{app:B6}

Нужно больше подразделов приложения!

\clearpage
\refstepcounter{chapter}
\addcontentsline{toc}{appendix}{\protect\chapternumberline{\thechapter}Чертёж детали}

\includepdf[pages=-]{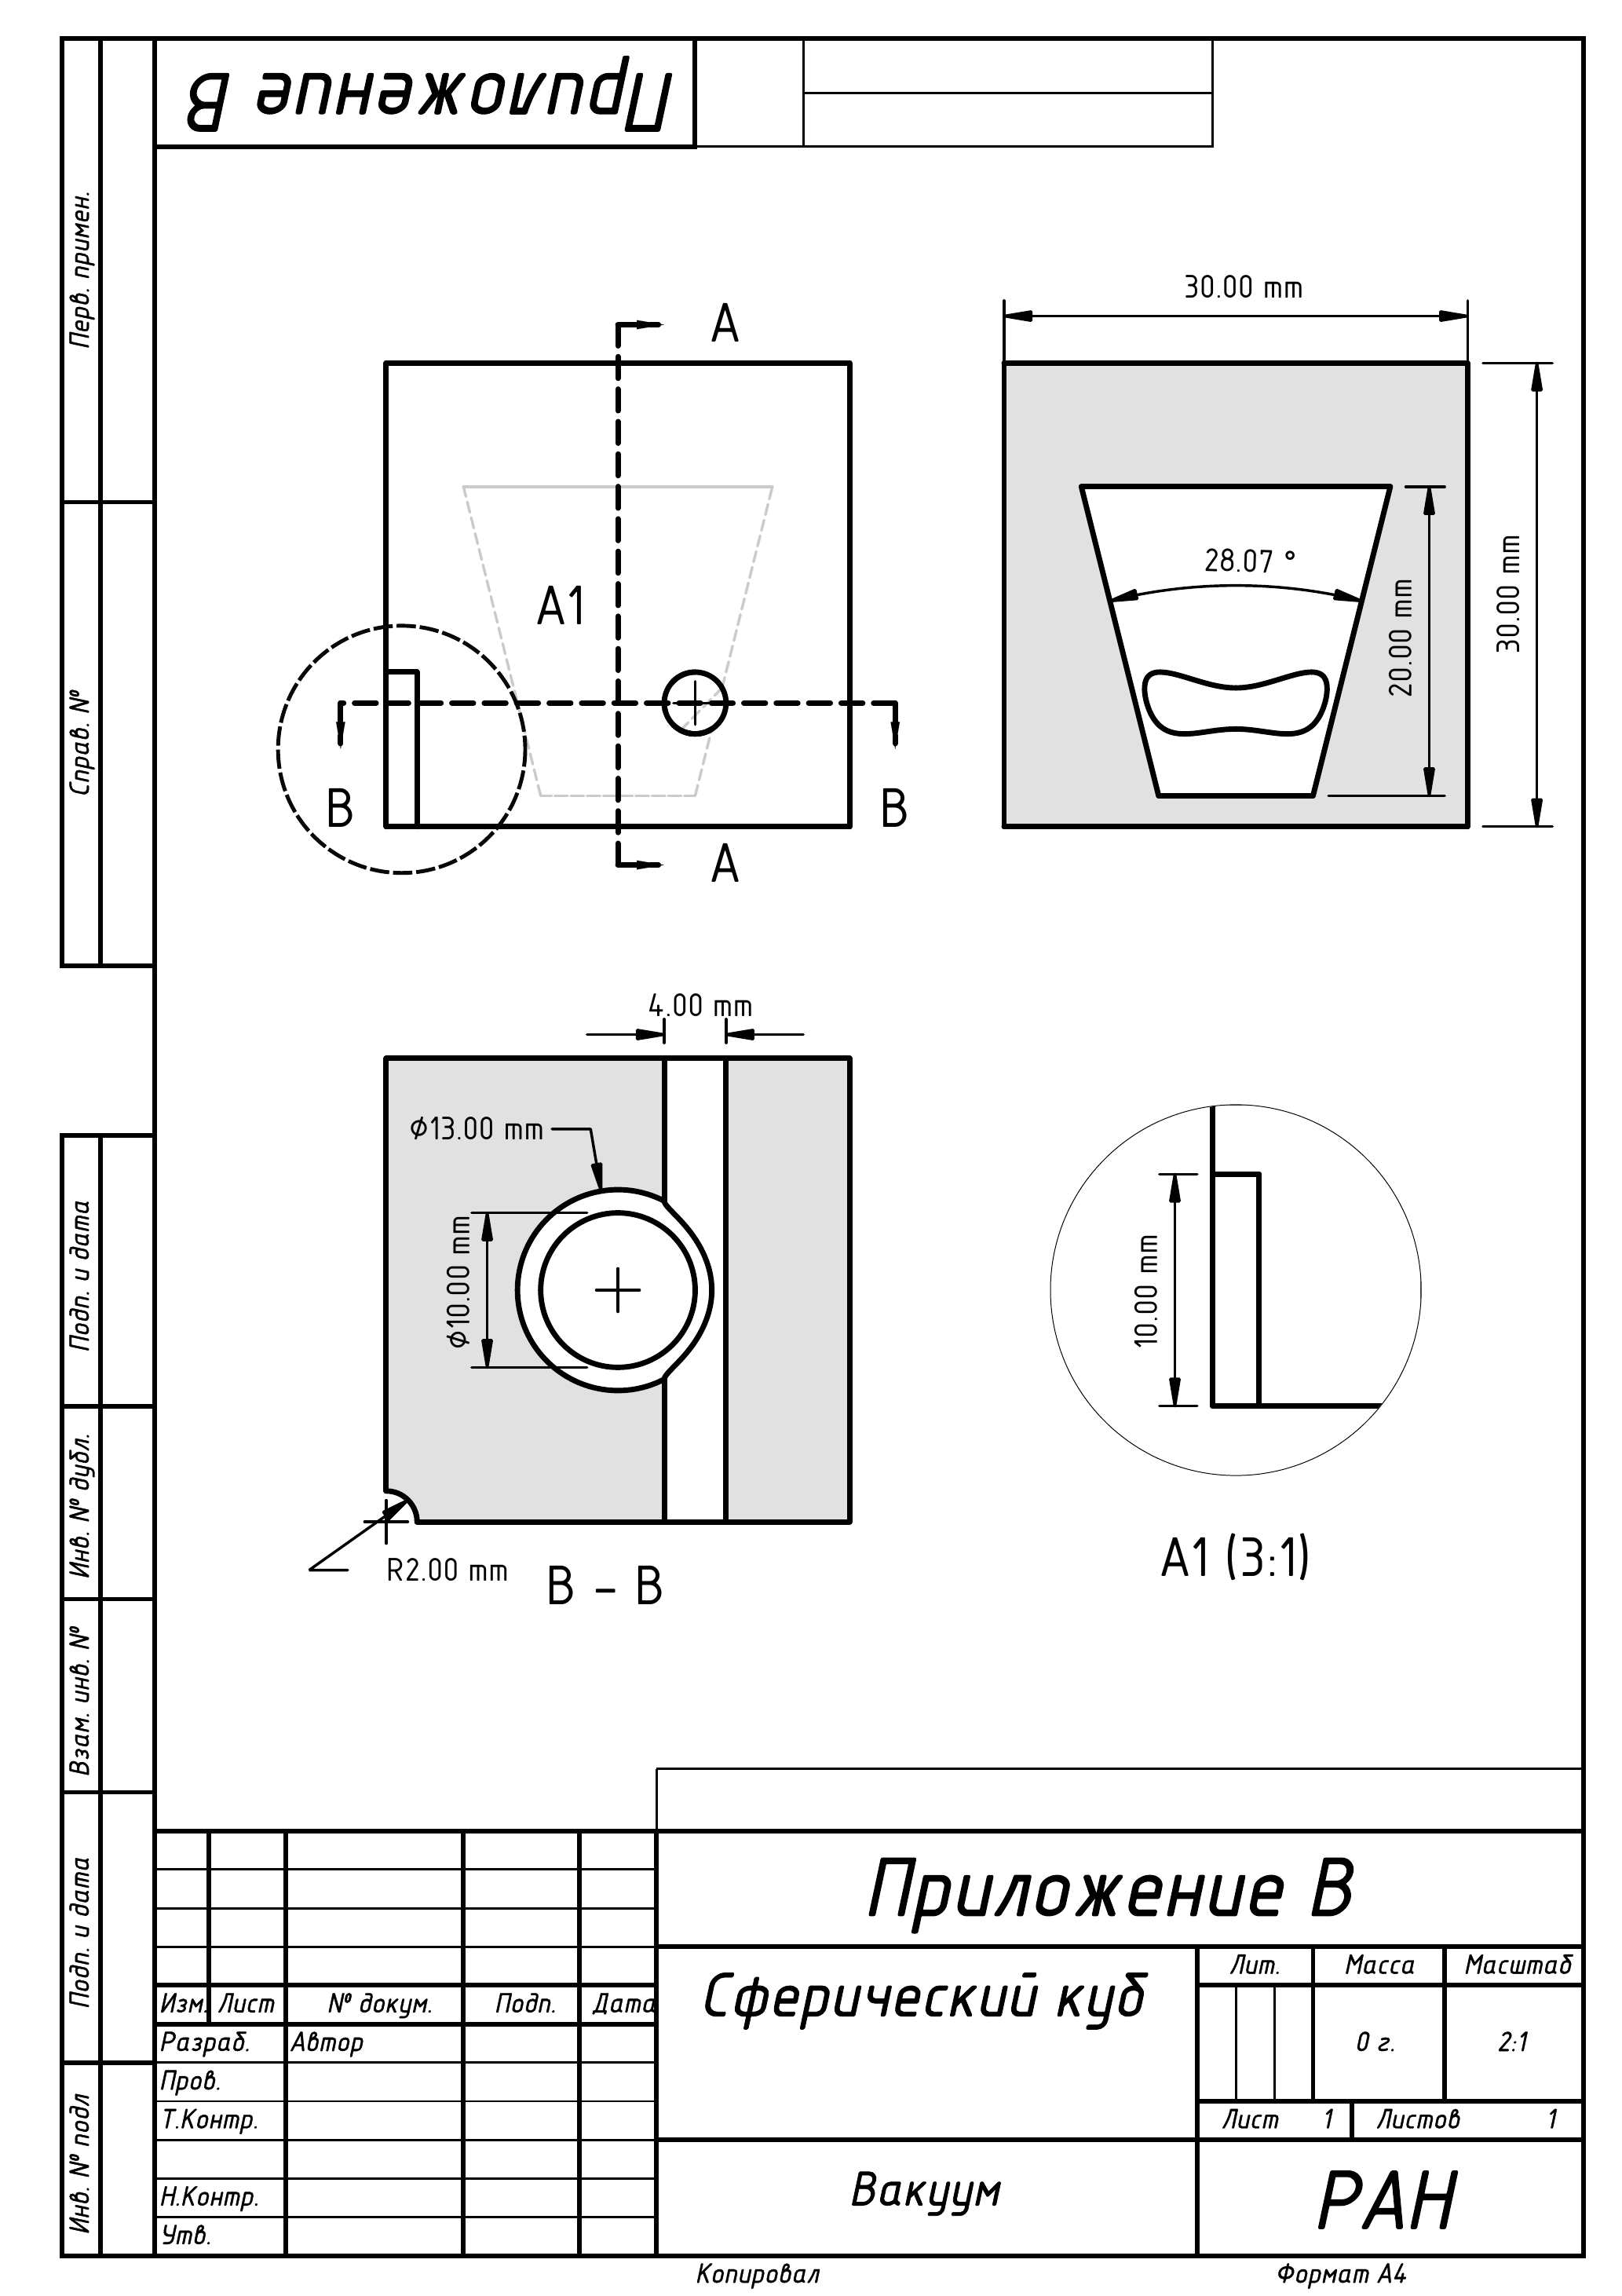}
